# Supplementary material for: Look Twice Before You Answer: Memory-Space Visual Retracing for Hallucination Mitigation in Multimodal Large Language Models
Source: arXiv:2410.03577 source file (2025-05-08)
Supplement: Supplementary file 1 [file legacy_appendix.tex]

\section{Appendix}\label{app:exp}
\subsection{Proof of robustness certification in
Theorem~\ref{theorem:robustness}}\label{app:robustness}
This section proves theoretical analysis on the robustness of HALC in approximating the 
optimal visual context $v^*$ via sampling in the FOV space 
(Theorem~\ref{theorem:robustness}). 
%
% First, we prove the instability of directly approximating $v^*$ with the grounding output 
% $v_d$ from the detector $\mathcal{G}_d$. 
% %
% Then we provide an analytical form of the expected deviation $\mathbb{E}[g(v^*, v_d)]$ 
% \jz{we changed the notation in main text}
% in the output distribution caused by detector perturbation $\eta$. 
%
With certain assumptions on $v^*$ and $v_d$, we focus on demonstrating the certified robustness on the decoding token probability distribution compared with that from the optimal visual context $v^*$, when sampling different FOVs based on $v_d$ which is initially determined by an detector $\mathcal{G}_d$.

The objective of HALC is to approximate the unknown optimal visual context for a decoding step, thereby mitigating hallucination and enhancing the truthfulness of the LVLM outputs.
We approach the optimal proxy by sampling a series of $n$ FOVs in the original image $v$, starting from $v_d$ according to some sampling function $\pi(\cdot|v_d)$.
We focus on bounding the minimum deviation of the decoding token probabilities from the optimum among the $n$ FOV samples, with the hope that we can always find some sample that is close to the optimal $v^*$ during this process. And as the sample size $n$ becomes larger, the minimum deviation becomes smaller, indicating that we can better cover the optimal visual context $v^*$ within the samples.\footnote{The subsequent selection of the best sample is another question, which is not concerned in this proof. We theoretically justify the existence of an ``optimal'' sample in the proof here, and HALC selects such a sample by contrasting FOV pairs based on the observation illustrated in \figref{fig:optimal_visual_context}.}

\jz{the use of certified robustness needs a bit more thinking}

% the minimum deviation of token probability from the optimal visual context on 
% two distinct instances of the sampling distribution $\pi(\cdot | v_d)$ within the set 
% $\Omega$, which represents the space of all distributions of potential visual contexts. 
% %

% The objective of HALC is to determine the most effective proxy within the discretized FOV 
% space that can closely approximate the optimal visual context, thereby mitigating 
% hallucination and enhancing the truthfulness of the LVLM outputs. 
% %
% Here, we focus on providing the proof for the certified robustness on the minimum deviation 
% of token probability from the optimal visual context.
%

\begin{proof}

% \jz{===== this beginning part, setting up assumptions,  will be updated after we sort out the correct proof =====}

Let $v^*=(w^*, h^*, p^*)$ be the optimal visual context, represented by a 3-tuple of its width, height, and center point.
The corresponding optimal token decoding probability distribution is $p_\theta(\cdot|v^*)$, where $\theta$ denotes the parameters of the LVLM {\lvlm}, and we ignore the condition on the textual query $x$ and previously generated tokens $y_{<t}$ for simplicity.
We rely on a symmetric discrepancy measure $D(\cdot,\cdot)\in [0, 1]$ to compare the disparity between two probability distributions, such as the Jensen-Shannon divergence, or the total variation distance.
We assume that the model prediction is robust around $v^*$ against small perturbations. In particular, we assume that there exists a tolerable small $\epsilon$-neighborhood $\mathcal{B}(v^*, \epsilon)=\{\hat{v}: \|\hat{v} - v^*\|\leq \epsilon\}$ around $v^*$, such that
\begin{equation}
    g(v^*, \hat{v}) = D(p_\theta(\cdot|v^*), D_\theta(\cdot|\hat{v})) \leq \delta\ll 1,\quad \forall \hat{v} \in \mathcal{B}(v^*, \epsilon)
\end{equation}
Essentially, for any visual context window (or FOV) close enough to $v^*$, the output token probability disparity is tiny, which is likely to result no difference in greedy decoding.

From the FOV detector $\mathcal{G}_d$, the output visual context is denoted as $v_d=(w_d, h_d, p_d)$, which is in general not the optimal.
We assume $v_d = v^* + \eta$ in the 3-tuple vector space, where $\eta$ is the perturbation vector from the optimal.
The detection perturbation is often large enough with $\|\eta\| > \epsilon$, making $v_d$ outside of the $\epsilon$-neighborhood of $v^*$.

$v_d \rightarrow v^*$:
If we directly use the detector output $v_d$ as an approximation of the optimal visual context $v^*$, the output distribution deviation from the optimum, measured by $g(v^*, v_d)$, is often unpredictable, when $v_d$ does not fall in the hypothetical tolerable region $\mathcal{B}(v^*, \epsilon)$.
An example can be seen as the inaccurate detection $v_d$ in \figref{fig:optimal_visual_context} results in the wrong token prediction \textit{book}.
This prompts the need for our proposed FOV sampling approach with the hope to find samples close to the optimal $v^*$.

\bfsection{$\pi(\cdot | v_d) \rightarrow v^*$:} 
Thus we consider sampling conditioned on $v_d$ in the discretized FOV space to enhance the 
robustness of optimal visual context approximation, hoping to find some sample that is close to the optimal. To do this, we obtain an upper bound on the minimum deviation from the output distribution among a collection of FOV samples.
Assume $\pi(\cdot | v_d) \in \Omega$ is an arbitrary sampling function conditional on the initial FOV detection $v_d$, where $\Omega$ 
denotes the sampling space over all potential visual contexts in the image. $\pi$ can either be a deterministic sampling function, or a stochastic sampling process with a probabilistic distribution over $\Omega$.
%
% Without loss of generality, we assume the the 
% %
Suppose we acquire $n$ samples $v_1, v_2, \ldots, v_n$ according to $\pi(\cdot|v_d)$, we denote the minimum deviation of the resulted token probability from that of the optimal visual context $v^*$ as
\begin{equation}
    h_{\pi}(v^*, n) = \min_{i=1,\ldots, n} D\left(p_{\theta}(\cdot | v^*), p_{\theta}(\cdot | v_i)\right)
\end{equation}
where $D$ is a symmetric discrepancy measure between two probability distributions, such as the Jensen-Shannon divergence, or the total variation distance, that is within the range of $[0, 1]$.
Having a small value of $h_{\pi}(v^*, n)$ would indicate that we can find some visual context that is close to the optimal $v^*$ through $n$ samples.

We proceed to estimate the minimum deviation $h_{\pi}(v^*, n)$ from the optimal visual 
context $v^*$ with $n$ samples.
We introduce a partition based on the occurrence 
of two probabilistic events: the event $A$ where at least one of the samples falls into the 
ball close to $v^*$, and its complement. 
Let us denote the probability of at least one sample falling within the ball \jz{formulate} as $P(A)$, and 
the complementary event's probability as $P(\neg A) = 1 - P(A)$. 
Hence, we can express the minimum divergence $h_{\pi}(v^*, n)$ as a marginalization over 
these events:
\begin{align}\label{eqn:expected_H}
h_{\pi}(v^*, n) &= P(A) \cdot [h_{\pi}(v^*, n) | A] + P(\neg A) \cdot [h_{\pi}(v^*, n) | \neg A]
\end{align}
Recognizing that for the one sample in the vicinity of $v^*$ in the event of $A$, its decoding token probability deviation from the optimal is bounded by $\delta\ll 1$ based on our assumption. Hence we have
\begin{align}\label{eq:general_bound}
    h_{\pi}(v^*, n) \leq & P(A) \cdot \delta + P(\neg A) \cdot 1 \leq  \delta + P(\neg A)
\end{align}

Next, we consider two instances of the sampling function $\pi(\cdot | v_d)$ that yield an upper bound for $h_{\pi}(v^*, n)$.

\bfsection{Normal Distribution Sampling.}
Suppose sampling from $\pi$ follows a stochastic process following a normal distribution around $v_d$. We denote this sampling process as $\pi_g(\cdot|v_d)\sim \mathcal{N}(v_d, \sigma^2 I)$, where we assume a variance of $\sigma^2$ for each element of the visual context representation (width, height, center) independently. \jz{note to myself: change the notation of normal and notation of a ball neighborhood} For $\tilde{v}\in \Omega$, the probability of sampling $\tilde{v}$ following the multivariate normal distribution is 
\[q(\tilde{v}; v_d, \sigma^2 I) = \frac{1}{\sqrt{(2\pi\sigma^2)^k}} \exp\left(-\frac{1}{2\sigma^2}(\tilde{v} - v_d)^\top (\tilde{v} - v_d)\right) \]
where $k=3$ is the dimension of the FOV representation vector.
The probability of event $\neg A$ happening, which is none of $n$ FOV samples falling within the $\epsilon$-neighborhood of $v^*$, is
\begin{align}
    P(\neg A) &= P(\|v_1 - v^*\| > \epsilon) \wedge P(\|v_2 - v^*\| > \epsilon) \wedge \cdots P(\|v_n - v^*\| > \epsilon) \\
    &= P(\|\tilde{v} - v^*\| > \epsilon) ^ n \\
    &= P(\|\tilde{v} - (v_d - \eta)\| > \epsilon) ^ n 
\end{align}
%
% \jz{note to myself: define $v_d=v^* + \eta$ earlier}
From the normal distribution assumption of $\tilde{v}$, we know that $\tilde{v} - (v_d - \eta)$ also follows a normal distribution $\mathcal{N}(\eta, \sigma I)$.
Therefore,
\begin{align}
    P(\neg A) &= \left(1 - P(\|\tilde{v} - (v_d - \eta)\| \leq \epsilon )\right) ^ n \\
    &= \left(1 - \int_{\nu: \|\nu\|\leq \epsilon} \frac{1}{\sqrt{(2\pi\sigma^2)^k}} \exp\left(-\frac{1}{2\sigma^2}(\nu - \eta)^\top (\nu - \eta)\right) d^k \nu \right) ^ n \\
    &= \left(1 - C_g(\epsilon, \eta)\right) ^ n
\end{align}
where we use $C_g(\epsilon, \eta)\in (0, 1)$ to denote the constant value given $\epsilon$ and $\eta$.
Following \eqnref{eq:general_bound}, we now have
\begin{align}
    h_{\pi_g}(v^*, n) \leq \delta + (1 - C_g(\epsilon, \eta))^n
\end{align}
where the second term goes to $0$ as $n$ is increasing to larger values.

\bfsection{Exponential Expansion Sampling.}
Now suppose sampling from $\pi$ follows an exponential expanding/shrinking process, where a sample can be expressed as $v_r=(w_r, h_r, p_r)=((1+\lambda)^r w_d, (1+\lambda)^r h_d, p_d)$ with an expanding factor $\lambda$ (assuming $\lambda >0$ without loss of generality) and some $r$. Essentially, the sample space comprises all fields of view (FOVs) that maintain the same aspect ratio (i.e. $w_d/h_d$) and the same center $p_d$ with $v_d$.  
Assume the sampling is uniform among all possible FOVs in the sample space, which we denote as $\pi_e(\cdot|v_d)\sim \mathcal{U}(r\in [r_{\min}, r_{\max}])$, where $r_{\min}$ and $r_{\max}$ correspond to the smallest FOV allowed (such as a few pixels) and the largest FOV possible (i.e. the entire original image v), respectively.

% For this sampling distribution, we further pose two mild assumptions on the initial detection $v_d$.
For this sampling distribution, we introduce two moderate assumptions regarding the initial detection $v_d$.
First, the center of the detection is relatively close to the optimum, such that $|p_d - p^*|<\epsilon$.
Second, The detection $v_d$ and the optimum $v^*$ share the same aspect ratio, meaning $w_d/h_d=w^*/h^*$.
This assumption is reasonable since the optimum is unknown, and we can assume it adheres to the aspect ratio used by a standard detector.

We begin by deriving the range of $r$ such that $v_r$ falls into the small neighborhood $\mathcal{B}(v^*, \epsilon)$ around $v^*$. We need
\begin{align}
    &\|v_r - v^*\| \leq \epsilon \\
    \implies\quad (w_r - w^*)^2 + &(h_r - h^*)^2 + (p_r - p^*)^2 \leq \epsilon^2 \\
    \implies\quad [(1+\lambda)^r w_d - w^*]^2 + &[(1+\lambda)^r h_d  - h^*]^2 + (p_d - p^*)^2 \leq \epsilon^2 \\
    % \implies\quad &\cdots \nonumber\\
    &\vdots \nonumber\\
    \implies\quad (w_d^2 + h_d^2)\left((1+\lambda)^r - \frac{w_d w^* + h_d h^*}{(w_d^2 + h_d^2)} \right)^2 &\leq \epsilon^2 - (p_d - p^*)^2 - \frac{h_d^2 {h^*}^2}{(w_d^2 + h_d^2)}(\frac{w_d}{h_d} - \frac{w^*}{h^*})^2 \\
    &= \epsilon^2 - (p_d - p^*)^2 >0
\end{align}
Denoting constants $C_a=\frac{\epsilon^2 - (p_d - p^*)^2}{(w_d^2 + h_d^2)}$ and $C_b=\frac{w_d w^* + h_d h^*}{(w_d^2 + h_d^2)}$, we get the range of $r$ such that $v_r\in \mathcal{B}(v^*, \epsilon)$ as
\begin{align}
    \max\left(r_{\min}, \frac{\log(C_b - \sqrt{C_a})}{\log(1+\lambda)}\right) &\leq r\leq \min\left(r_{\max}, \frac{\log(C_b + \sqrt{C_a})}{\log(1+\lambda)}\right)\quad\quad \text{if}\quad C_b > \sqrt{C_a} \\
    \text{Or}\hspace{1.5in} r_{\min} &\leq r\leq \min\left(r_{\max}, \frac{\log(C_b + \sqrt{C_a})}{\log(1+\lambda)}\right)\quad\quad \text{if}\quad C_b \leq \sqrt{C_a}
\end{align}
% Or
% \begin{align}
%     r_{\min} \leq r\leq \min\left(r_{\max}, \frac{\log(C_b + \sqrt{C_a})}{\log(1+\lambda)}\right)\quad\quad \text{if}\quad C_b \leq \sqrt{C_a} 
% \end{align}
%
We further denote this range as $r\in[C_{\min}(\epsilon, v^*, v_d), C_{\max}(\epsilon, v^*, v_d)]$, with $r_{\min}\leq C_{\min}(\epsilon, v^*, v_d) < C_{\max}(\epsilon, v^*, v_d)\leq r_{\max}$.
Based on the independent uniform sampling assumption, the probability of the event $\neg A$ that none of the $n$ samples fall into the $\epsilon$-neighborhood around the optimum $\mathcal{B}(v^*, \epsilon)$ is
\begin{equation}
    P(\neg A) = \left(1-\frac{C_{\max}(\epsilon, v^*, v_d) - C_{\min}(\epsilon, v^*, v_d)}{r_{\max} - r_{\min}}\right)^n = \left(1-C_e(\epsilon, v^*, v_d)\right)^n
\end{equation}
where we use $C_e(\epsilon, v^*, v_d)\in(0, 1]$ to denote the constant value depending on $\epsilon, v^*, v_d$.
Following \eqnref{eq:general_bound}, we then have
\begin{equation}
    h_{\pi_e}(v^*, n) \leq \delta + (1 - C_e(\epsilon, v^*, v_d)))^n
\end{equation}
where the second term goes to 0 as $n$ is increasing to larger values.

\bfsection{Discussion.}
In the above, we demonstrated that beginning with the initial detected visual context $v_d$, under certain mild conditions, acquiring $n$ samples according to a distribution $\pi(\cdot|v_d)$ is an efficient method for identifying a sample that leads to a small bounded deviation in the token decoding probabilities from those derived from the optimal visual context $v^*$.
The more samples acquired, the tighter the bound is.  
This provides a simple and robust way of approximating the optimum.

Different sampling distributions have distinct characteristics.
For normal distribution sampling $\pi_g(\cdot|v_d)\sim\mathcal{N}(v_d, \sigma^2 I)$, the variance parameter $\sigma^2$ determines the spread of the samples and thus the likelihood of approximating the optimal $v^*$ within $\mathcal{B}(v^*, \epsilon)$.
For exponential expansion sampling $\pi_e(\cdot|v_d)\sim\mathcal{U}(r\in[r_{\min}, r_{\max}])$ with samples $v_r=((1+\lambda)^r w_d, (1+\lambda)^r h_d, p_d)$, the parameter $\lambda$ controls the rate of growth for the sampled visual contexts. In practice, we apply discrete integer values of $r$ to acquire different samples efficiently, thus $\lambda$ affects the sample coverage of the visual information around $v^*$.

The choice of the sampling distribution $\pi$ is contingent upon factors such as the quality of the detector $\mathcal{G}_d$, the LVLM backbone {\lvlm}, the textual query $x$, and the visual input $v$.
Specifically, the continuous normal distribution is advantageous for concentrated sampling around $v_d$, which is particularly effective when the detection perturbation $\eta$ is small (meaning $v_d$ is near $v^*$).
In contrast, exponential expansion sampling covers an extended range of visual contexts quickly, which is preferable when limited context information is obtained.
In scenarios where significant underestimation or overestimation in $G_d$ detection is present, the exponential expanding strategy can discover the optimal visual context more effectively. 
\end{proof}

\subsection{Experimentation Details}\label{app:exp}
\subsubsection{Experimental Setups}\label{app:hyper}
The overall experiment settings is reported in \tabref{tab:hyperparameter_overall}. 
While the regular greedy decoding follows this setting, the beam search variant in our 
experiment essentially applies a token-wise beam search based on accumulated probability 
scores of the previous tokens $y_{<t}$. 
We use the default code for implementation of these two baselines in HuggingFace TransformersRepository~\cite{wolf2020transformers}.\footnote{\url{https://huggingface.co/docs/transformers}}

\begin{table}[H]
\centering
\caption{Overall Experiment Settings}
\begin{tabular}{l|c}
\hline
\textbf{Parameters} & \textbf{Value} \\ \hline
Maximum New Tokens (CHAIR) & $64$  \\ \hline
Maximum New Tokens (POPE)  & $64$  \\ \hline
Maximum New Tokens (MME)  & $128$ \\ \hline
Top-k & False \\ \hline
Top-p & $1$ \\ \hline
Temperature $\tau$ & $1$ \\ \hline
\end{tabular}
\label{tab:hyperparameter_overall}
\end{table}

The complete hyper-parameters for HALC in our experiments in \secref{sec:experiments} is 
reported in 
\tabref{tab:hyperparameter_halc}. Specifically, there are four major hyper-parameters that 
can actively adjust the effectiveness of HALC to adapt to different task settings:
\begin{enumerate}
    \item \textit{FOV Sampling Distribution}: Typically, a normal distribution, which concentrated around ${v}_d$, provides a tighter bound under minimal perturbations, while an exponential distribution, with a more averaged coverage of the sampling space, is preferable when less contexts of the task is available. Thus to preserve generality in our experiment, we have employed the exponential distribution with exponential growth factor $\lambda=0.6$.
    \item \textit{Number of Sampled FOVs $n$}: $n$ determines the number of sampled FOVs in the discretized FOV space. According to Theorem~\ref{theorem:robustness}, while increasing $n$ and adjusting the distribution parameters can efficiently reduce $C_S$ and enhance the robustness against bounded perturbations, it's notable that the runtime costs also raise with $n$. Consequently, we set $n=4$ across all our experiments.
    \item \textit{JSD Buffer Size $m$}: For each beam in the overall beam search process (beam size $k$), our bi-adaptive visual grounding module samples $n$ visual contexts, which through interpolated JSD calculation would produce $\frac{n \cdot (n-1)}{2}$ JSD values in total. Then we select the top $m$ FOV pairs with relatively large discrepancy to produce contrastive candidate distributions.
    \item \textit{Beam Size $k$}: The beam size $k$ is set to adjust the diversity and range for HALC to search for the best candidate captions. Essentially, the global visual matching score module selects the top $k$ diverse captions from $2m \cdot k$ text sequence candidates passed from the local adaptive visual grounding module. While a larger $k$ involves a larger search space and hopefully a better generation, the runtime cost also raises linearly w.r.t. $k$. HALC adopts Bootstrapping Language-Image Pre-training (BLIP)~\cite{li2022blip} for both text and image encoding when computing their cosine similarity scores. Notably given the global search capability of our visual matching score module, HALC seeks to preserve a more diverse set of captions within the beam buffer.
    \item \textit{Other Hyperparameters}: Our implementation inherits an additional 
    hyperparameter, adaptive plausibility threshold, originally 
    from DoLA~\citep{chuang2023dola}. 
\end{enumerate}
%
% \rv{Typically, a normal distribution, which concentrated around $\tilde{v}_d$, provides a tighter bound under minimal perturbations, 
% while an exponential distribution, with a more averaged coverage of the sampling space, is preferable when less priors of the task is 
% available.}
%
\begin{table}[H]
\caption{HALC Hyperparameter Settings}
\centering
\begin{tabular}{l|c}
\hline
\textbf{Parameters} & \textbf{Value} \\ \hline
Amplification Factor $\alpha$ & $0.05$  \\ \hline
JSD Buffer Size $m$ & $6$  \\ \hline
Beam Size & $1$ \\ \hline
FOV Sampling & Exponential Expanding  \\ \hline
Number of Sampled FOVs $n$  & $4$  \\ \hline
Exponential Growth Factor $\lambda$ & 0.6\\ \hline
Adaptive Plausibility Threshold & $0.1$ \\
\hline
\end{tabular}
\label{tab:hyperparameter_halc}
\end{table}

Regarding the comparison of HALC with SOTAs that are specifically designed for OH mitigation, we 
adopt the code, hyper-parameters, and pre-trained models of each method outlined in their 
public repositories and papers respectively. 
Specifically, the hyper-paratermers for DoLa~\cite{chuang2023dola}\footnote{\url{https://github.com/voidism/DoLa}} 
is reported in \tabref{tab:hyperparameter_dola}; 
OPERA~\cite{huang2023opera}\footnote{\url{https://github.com/shikiw/OPERA}} 
is reported in \tabref{tab:hyperparameter_opera}; 
and the hyperparatermers for 
VCD~\cite{leng2023mitigating}\footnote{\url{https://github.com/DAMO-NLP-SG/VCD}} is 
reported in \tabref{tab:hyperparameter_vcd}. 
For each of these baselines, we strictly follow their implementations and hyper-parameters 
as reported in the paper to reproduce their results.
\begin{table}[H]
\caption{DoLa Hyperparameter Settings}
\centering
\begin{tabular}{l|c}
\hline
\textbf{Parameters} & \textbf{Value} \\ \hline
Repetition Penalty $\theta$ & $1.2$  \\ \hline
Adaptive Plausibility Threshold $\beta$ & $0.1$\\ \hline
Pre-mature Layers & $[0, 2 \cdots, 32]$\\
\hline
\end{tabular}
\label{tab:hyperparameter_dola}
\end{table}
\begin{table}[H]
\caption{OPERA Hyperparameter Settings}
\centering
\begin{tabular}{l|c}
\hline
\textbf{Parameters} & \textbf{Value} \\ \hline
Self-attention Weights Scale Factor $\theta$ & $50$  \\ \hline
Attending Retrospection Threshold & $15$\\\hline
Beam Size & $3$\\
\hline
Penalty Weights & $1$\\
\hline
\end{tabular}
\label{tab:hyperparameter_opera}
\end{table}
\begin{table}[H]
\caption{VCD Hyperparameter Settings}
\centering
\begin{tabular}{l|c}
\hline
\textbf{Parameters} & \textbf{Value} \\ \hline
Amplification Factor $\alpha$ & $1$  \\ \hline
Adaptive Plausibility Threshold & $0.1$\\\hline
Diffusion Noise Step & $500$\\
\hline
\end{tabular}
\label{tab:hyperparameter_vcd}
\end{table}

Regarding post-hoc correction method woodpecker~\cite{yin2023woodpecker}\footnote{\url{https://github.com/BradyFU/Woodpecker}}  and LURE~\cite{zhou2023analyzing}\footnote{\url{https://github.com/YiyangZhou/LURE}} , we also strictly follow their implementations and hyper-parameters 
as reported in the paper to reproduce their results. For woodpecker, we adopt their original code and use OpenAI API to access GPT-3.5 Turbo. In average, per 500 images would result in approximately \$4.5 cost. For LURE, we also directly adopt their pre-trained projection layer model (for Minigpt4) to reproduce the results reported in this paper. All the hyper-parameters are default.

\subsubsection{Empirical Studies on Optimal Visual Contexts}\label{app:contexts}

We verify our insight that optimal visual context is important in correcting object hallucination through an empirical pilot study. 
\figref{fig:pattern_analysis} shows the oracle performance of OH levels when we 
rely on optimal visual contexts for tokens through brute-force search, with greedy decoding 
on the MME benchmark~\cite{fu2023mme} on three categories of 
OH. Specifically, each MME sub-task contains 30 images, and we have followed~\cite{leng2023mitigating} and selected four sub-tasks (including \textit{existence}, \textit{count}, \textit{color}, \textit{position}) to evaluate the hallucination in our analysis, in total 110 distinct images. Based on these images, we manually constructed multiple challenging questions (2-4 per image) that are likely to induce the LVLM to hallucinate (e.g. some minor objects in the distance or some plausible but unfaithful objects that are likely to co-occur). Then we take each question as a count unit and calculate the number of hallucinations on word level (instead of token level) which could attributed for each of the 3 sources. Then for each question with a hallucination occurring, we search across the original image input using a brutal-force breadth-first algorithms until the hallucinating token can be corrected to be consistent with the ground truth. This process effectively succeed to retrieve the optimal visual context for 54.0\% of the questions. For those questions that fail this brutal-force search, we further manually select the visual context candidates based on human priors. In total, 84.5\% of the questions that contain these three sources of hallucinations can be eliminated with an explicit optimal visual prior $v^*$.

\subsection{MME Experiment Details}\label{app:mme}

The experiment details mostly follow Appendix~\ref{app:contexts}, where we adopt each sub-task of 30 images from MME dataset, and reconstruct the question prompt following OPOPE. Specifically, instead of simply asking a yes/no question, we first ask the decoder to generate a detailed caption then check whether the MME-targeted
positive/negative word existed in the caption. The detailed results are reported in Table~\ref{tab:MME_result}.

\begin{table}[h!]
\centering
\caption{Comparison of Decoder Performances on 4 MME sub-tasks}
\label{table:decoder_performance}
\begin{tabular}{@{}lcccccc@{}}
\toprule
Decoder & Existence & Position & Color & Count & Max Tokens & Num of Samples \\
\midrule
HALC  & 155 & 73.33 & 141.67 & 93.33 & 128 & 110 \\
Greedy & 145 & 63.33 & 118.33 & 85 & 128 & 110 \\
DoLa   & 145 & 60    & 118.33 & 85 & 128 & 110 \\
Opera  & 135 & 56.67 & 115    & 80 & 128 & 110 \\
VCD    & 135 & 70    & 133.33 & 70 & 128 & 110 \\
LURE   & 140 & 60    & 108.33 & 68.33 & 128 & 110 \\
\bottomrule
\label{tab:MME_result}
\end{tabular}
\end{table}

\newpage
\subsection{Comprehensive POPE Results}\label{app:pope}
\begin{table}[H]
\addtolength{\tabcolsep}{8pt}  % column
  % row
\fontsize{8pt}{8pt}\selectfont
\centering
\caption{Detailed OPOPE results with random, popular and adversarial samplings.}
%\resizebox{\linewidth}{!}{
\begin{tabular}{l l l l l l l}
\toprule
\textbf{Setting} & \textbf{Model} & \textbf{Decoding} & \textbf{Accuracy} & \textbf{Precision} & \textbf{Recall} & \textbf{$F_\text{0.2}$ Score} \\ 
\midrule
\multirow{12}{*}{Random} 
& \multirow{6}{*}{MiniGPT-4} & Greedy & 68.30 & 97.24 & 37.67 & 91.67 \\
&                          &Beam Search & 68.37 & 96.30 & 38.20 & 90.98 \\
&                          & DoLa     & 68.50 & 97.27 & 38.07 & 91.78 \\
&                          & OPERA   & 68.67 & 96.98 & 38.53 & 91.63 \\
&                          & VCD     & 67.10 & 96.22 & 35.60 & 90.30 \\
&                          & Woodpecker   & 69.07 & 96.99 & 39.366 & 91.83\\
&                          & LURE   & 69.50 & 96.65 & 40.4 & 86.76 \\
&                          & HALC    & 67.90 & 97.36 & 40.4 & 91.74 \\ \cline{2-7}
& \multirow{6}{*}{LLaVA-1.5} & Greedy & 72.20 & 97.17 & 45.73 & 93.14 \\
&                          & Beam Search  & 71.33 & 97.48 & 43.80 & 93.09 \\
&                          & DoLa     & 72.30 & 96.78 & 46.13 & 92.86 \\
&                          & OPERA   & 71.20 & 96.76 & 43.87 & 92.47 \\
&                          & VCD     & 72.07 & 96.89 & 45.60 & 92.87 \\
&                          & Woodpecker   & 70.83 & 95.89 & 43.53 & 91.65\\
&                          & LURE   & 71.67 & 97.24 & 44.6 & 93.02\\
&                          & HALC    & 71.87 & 97.86 & 44.73 & 93.58 \\ \cline{2-7}
& \multirow{6}{*}{mPLUG-Owl2} & Greedy & 71.27 & 96.91 & 43.93 & 92.62 \\
&                          & Beam Search     & 70.50 & 97.26 & 42.20 & 92.61 \\
&                          & DoLa     & 71.47 & 96.92 & 44.33 & 92.69 \\
&                          & OPERA   & 70.17 & 96.92 & 41.67 & 92.22 \\
&                          & VCD     & 70.93 & 97.31 & 43.07 & 92.81 \\
&                          & Woodpecker   & 70.27 & 97.99 & 41.38 & 93.09\\
&                          & LURE   & 70.83 & 96.71 & 43.13 & 92.30 \\
&                          & HALC    & 71.50 & 97.38 & 44.20 & 93.07 \\ \cline{1-7}
\multirow{12}{*}{Popular} 
& \multirow{6}{*}{MiniGPT-4} & Greedy & 66.43 & 88.70 & 37.67 & 84.30 \\
&                          & Beam Search     & 67.00 & 90.09 & 38.20 & 85.62 \\
&                          & DoLa     & 66.8 & 89.50 & 38.07 & 85.08 \\
&                          & OPERA   & 66.80 & 88.65 & 38.53 & 84.43 \\
&                          & VCD     & 65.47 & 65.47 & 35.60 & 83.64 \\
&                          & Woodpecker   & 67.37 & 89.47 & 39.37 & 85.29 \\
&                          & LURE   & 67.8 & 89.38 & 40.4 & 85.40 \\
&                          & HALC    & 66.37 & 90.02 & 36.80 & 85.27 \\ \cline{2-7}
& \multirow{6}{*}{LLaVA-1.5} & Greedy & 70.27 & 89.79 & 45.73 & 86.58 \\
&                          & Beam Search  & 69.80 & 91.25 & 43.8 & 87.6 \\
&                          & DoLa     & 70.43 & 89.75 & 46.13 & 86.60 \\
&                          & OPERA   & 69.63 & 90.51 & 43.87 & 86.95 \\
&                          & VCD     & 70.57 & 91.08 & 45.60 & 87.71 \\
&                          & Woodpecker   & 69.37 & 90.07 & 43.53 & 86.51 \\
&                          & LURE   & 69.63 & 89.32 & 44.6 & 86.00 \\
&                          & HALC    & 70.03 & 90.74 & 44.67 & 87.28 \\ \cline{2-7}
& \multirow{4}{*}{mPLUG-Owl2} & Greedy & 69.30 & 89.13 & 43.93 & 85.74 \\
&                          & Beam Search     & 68.83 & 90.27 & 42.20 & 86.48 \\
&                          & DoLa     & 69.53 & 89.35 & 44.33 & 85.99 \\
&                          & OPERA   & 69.03 & 92.02 & 41.67 & 87.94 \\
&                          & VCD     & 69.43 & 91.10 & 43.07 & 87.35 \\
&                          & Woodpecker   & 68.58 & 90.73 & 41.38 & 86.75 \\
&                          & LURE   & 69.17 & 89.99 & 43.13 & 86.38 \\
&                          & HALC    & 69.63 & 89.95 & 44.20 & 86.50 \\ \cline{1-7}
\multirow{12}{*}{Adversarial} 
& \multirow{6}{*}{MiniGPT-4} & Greedy & 65.60 & 85.35 & 37.67 & 81.38 \\
&                          & Beam Search     & 66.3 & 87.21 & 38.20 & 83.11 \\
&                          & DoLa     & 65.87 & 85.74 & 38.07 & 81.80 \\
&                          & OPERA   & 66.3 & 86.66 & 38.53 & 82.68 \\
&                          & VCD     & 64.77 & 85.44 & 35.60 & 81.08 \\
&                          & Woodpecker   & 66.88 & 87.53 & 39.37 & 83.60 \\
&                          & LURE   & 67.13 & 86.82 & 40.4 & 83.14\\
&                          & HALC    & 66.00 & 88.47 & 36.80 & 83.94 \\ \cline{2-7}
& \multirow{6}{*}{LLaVA-1.5} & Greedy & 69.23 & 86.30 & 45.73 & 83.44 \\
&                          & Beam Search     & 68.47 & 86.45 & 43.8 & 83.33 \\
&                          & DoLa     & 69.33 & 86.07 & 46.13 & 83.30 \\
&                          & OPERA   & 68.37 & 86.01 & 43.87 & 82.95 \\
&                          & VCD     & 69.37 & 86.91 & 45.60 & 83.99 \\
&                          & Woodpecker   & 69.20 & 89.45 & 43.53 & 85.96 \\
&                          & LURE   & 68.7 & 86.1 & 44.6 & 83.13 \\
&                          & HALC    & 69.87 & 90.21 & 44.67 & 86.80 \\ \cline{2-7}
& \multirow{6}{*}{mPLUG-Owl2} & Greedy & 68.73 & 87.16 & 43.93 & 83.98 \\
&                          & Beam Search     & 68.27 & 88.17 & 42.20 & 84.63 \\
&                          & DoLa     & 68.87 & 87.02 & 44.33 & 83.91 \\
&                          & OPERA   & 68.57 & 90.22 & 41.67 & 86.35 \\
&                          & VCD     & 69.07 & 89.69 & 43.07 & 86.10 \\
&                          & Woodpecker   & 67.85 & 87.94 & 41.38 & 84.29\\
&                          & LURE   & 67.73 & 84.91 & 43.13 & 81.86\\
&                          & HALC    & 69.23 & 88.50 & 44.20 & 85.21 \\
\bottomrule
\end{tabular}%
%}
\label{tab:pope_results}
\end{table}
%

% \newpage
% \subsection{MME Experiment Details}\label{app:mme}

\newpage
\subsection{Experiment Results on LLaVA-Bench}\label{app:llava_bench}
As discussed in \secref{subsec:llava_bench}, we leverage LLaVA-Bench~\cite{liu2023improved} 
as a case study to qualitatively compare the decoding outputs of HALC with other methods.
Results generated by HALC and other OH reduction baselines incorporating 
mPLUG-Owl2~\cite{ye2023mplug}, MiniGPT-4~\cite{zhu2023minigpt, chen2023minigpt}, and
LLaVA~\cite{liu2023visual} LVLM backbones are shown in 
\figref{fig:llava_bench_mplug},~\ref{fig:llava_bench_minigpt4} and~\ref{fig:llava_bench_llava}
respectively.
In all the plots, red fonts indicate OH, including any of the object existence, attribute or
relationship hallucinations.
\begin{figure}[h]
    \centering
    \includegraphics[width=0.85\textwidth]{Figures/mplug_llava_bench.pdf}
    \caption{
        LLaVA-Bench results comparing HALC and other methods with mPLUG-Owl2~\cite{ye2023mplug}
        backbone.
    }
    % }
    \label{fig:llava_bench_mplug}
    \vspace{-0.15in}
\end{figure}

\begin{figure}[t]
    \centering
    \includegraphics[width=0.7\textwidth]{Figures/minigpt4_llava_bench.pdf}
    \caption{
        LLaVA-Bench results comparing HALC and other methods with 
        MiniGPT-4~\cite{zhu2023minigpt, chen2023minigpt} backbone.
    }
    \label{fig:llava_bench_minigpt4}
    \vspace{-0.15in}
\end{figure}

\begin{figure}[t]
    \centering
    \includegraphics[width=0.75\textwidth]{Figures/llava_llava_bench.pdf}
    \caption{
        LLaVA-Bench results comparing HALC and other methods with LLaVA~\cite{liu2023visual}
        backbone.
    }
    % \jz{to be updated: change bars and legend}
    % }
    \label{fig:llava_bench_llava}
    \vspace{-0.15in}
\end{figure}
